# Supplementary material for: A method for Selecting Scenes and Emotion-based Descriptions for a Robot's Diary
Source: arXiv:2309.01951 source file (2023-09-05)
Supplement: Supplementary file 1 [file appendix.tex]

\section*{APPENDIX}

Appendixes should appear before the acknowledgment.
